# Supplementary material for: Refinement of Interval Approximations for Fully Commutative Quivers
Source: arXiv:2310.03649 source file (2023-11-13)
Supplement: Supplementary file 1 [file 999appendix.tex]

\appendix
\section{Symmetric functor $\sigma$ on $\mathcal{N}$}\label{appendix:sec1}

Recall the $\sigma$ functor we defined at example \ref{exa:sigma}. In this part we will going to list all the correspondence it gives us explicitly.

The Auslander-Reiten quiver for CL(4) (type \textit{fff}) can be found at page 56, Fig.17 of the paper \textit{Persistence Modules on Commutative Ladders of Finite Type}. We follow the numbering as in the note \textit{CL(4)に対する完全分解アルゴリズム（スケッチ）}(2021-05-07のセミナー) up to $11$, with numbering after 11 goes up symmetrically as they goes down from 10 to 1. This ordering has the advantage that $\sigma(N_{11+k})=N_{11-k}$ for $k=1,\cdots,10$.

An illustration of this numbering can be found \href{https://brave-northcutt-4bb316.netlify.app/ar}{here}.  

For convenience, we note down the pairs of non-intervals within which one is mapped to the other under $\sigma$:
\begin{multicols}{3}
\begin{itemize}
    \item $N_1\ \Leftrightarrow\ N_{21}$
    \item $N_2\ \Leftrightarrow\ N_{20}$
    \item $N_3\ \Leftrightarrow\ N_{19}$
    \item $N_4\ \Leftrightarrow\ N_{18}$
    \item $N_5\ \Leftrightarrow\ N_{17}$
    \item $N_6\ \Leftrightarrow\ N_{16}$
    \item $N_7\ \Leftrightarrow\ N_{15}$
    \item $N_8\ \Leftrightarrow\ N_{14}$
    \item $N_9\ \Leftrightarrow\ N_{13}$
    \item $N_{10}\ \Leftrightarrow\ N_{12}$
    \item $N_{11}\  \rotatebox[origin=c]{90}{$\circlearrowleft$}$
\end{itemize}
\end{multicols}

According to the arguments in section one, we have
\[
\delta^*_{N_{11+k}}(I)
=\delta^*_{\sigma(N_{11-k})}(I)
=\delta^*_{N_{11-k}}(\sigma(I)) 
\quad \forall I\in\mathcal{I},\ k=1,\cdots,11. 
\]

This allows us to obtain the values for $N_{12},N_{13},\cdots,N_{21}$ as long as we have the $\sigma$ map on each interval determined. This relationship can be determined easily from the AR-quiver as well, because each interval is mapped to its reflection along the middle line. 

However, we will not numbering the intervals using the AR-quiver. In order to to facilitate the input of matrix coefficients, the numbering provided in the demo is adopted. Below we list the pairs of values, with form designed to be compatible with the table in the demo.

\begin{tabular}{|c|c|c|c|c|c|c|c|c|c|c|c|}
%\hhline{|=|=|=|=|=|=|=|=|=|=|=|=|}
\hline\hline
     1, 20& 
     2, 19& 
     3, 18& 
     4, 17&
     5, 14& 
     6, 13& 
     7, 8& 
     8, 7&
     9, 16& 
     10, 15& 
     11, 12& 
     12, 11\\\hline
     13, 6&
     14, 5&
     15, 10&
     16, 9&
     17, 4&
     18, 3&
     19, 2&
     20, 1&
     21, 55&
     22, 54&
     23, 50&
     24, 40\\\hline
     25, 53&
     26, 49&
     27, 39&
     28, 46&
     29, 36&
     30, 30&
     31, 52&
     32, 48&
     33, 38&
     34, 45&
     35, 35&
     36, 29\\\hline
     37, 43&
     38, 33&
     39, 27&
     40, 24&
     41, 51&
     42, 47&
     43, 37&
     44, 44&
     45, 34&
     46, 28&
     47, 42&
     48, 32\\\hline
     49, 26&
     50, 23&
     51, 41&
     52, 31&
     53, 25&
     54, 22&
     55, 21&
     &
     &
     &
     &
     \\\hline
\end{tabular}
